# Supplementary material for: CARE: Ensemble Adversarial Robustness Evaluation Against Adaptive Attackers for Security Applications
Source: arXiv:2401.11126 source file (2024-01-20)
Supplement: Supplementary file 1 [file 9-appendix-attack.tex]

\section{Abbreviations and Acronyms}

\begin{table}[]
    \caption{Abbreviations and Acronyms}
    \begin{center}
    \begin{tabular}{@{}cccc@{}}
    \toprule
                                                                                &                                                                                      & AEs       & Adversarial Examples                     \\ 
            \multirow{2}{*}{\textbf{Terms}}                                    &                                                                                      & AT        & Adversarial Training                     \\
                                                                               &                                                                                      & MA-AT        & Multi-attack AT                     \\
                                                                               &                                                                                      & TE-AT        & Transfer Ensemble AT                     \\ \cmidrule(r){1-4}
                                                                             & \multirow{6}{*}{\begin{tabular}[c]{@{}c@{}}Gradient\\ -based\\ Attacks\end{tabular}} & FGSM      & Fast Gradient Sign Method                \\
                                                                               &                                                                                      & PGD       & Projected Gradient Descent               \\
                                                                               &                                                                                      & C\&W      & Carlini and Wagner Attack                \\
                                                                               &                                                                                      & JSMA      & Jacobian-based Saliency Map Attack       \\
                                                                               &                                                                                      & DF        & DeepFool Attack                          \\
                                                                               &                                                                                      & BIM       & Basic Iterative Method                                      \\ \cmidrule(r){2-4}
    \textbf{Attacks}                                                                              & \multirow{6}{*}{\begin{tabular}[c]{@{}c@{}}Gradient\\ -free\\ Attacks\end{tabular}}  & ZOO       & Zeroth-order Optimization                \\
                                                                               &                                                                                      & NES       & Natural Evolutionary Strategies          \\
                                                                               &                                                                                      & ZOSGD     & Zeroth-Order Stochastic GD \\
                                                                               &                                                                                      & ZOAda     & Zeroth-Order Adaptive Momentum    \\
                                                                               &                                                                                      & BA        & Boundary Attack                          \\
                                                                               &                                               & HSJA      & HopSkipJumpAttack                        \\ \cmidrule(r){2-4}
                                                                               &                      \multirow{3}{*}{\begin{tabular}[c]{@{}c@{}}Ensemble\\ Attack\end{tabular}}                                                                 & Avg-EA    & Average Ensemble Attack                     \\
                                                                               &                                                                                      & Max-EA    & Maximum Ensemble Attack                     \\
                                                                               &                                                                                      & Adp-EA    & Adaptive Ensemble Attack                    \\\cmidrule(r){1-4}
    \multirow{10}{*}{\textbf{Defenses}}                                                 & \multirow{3}{*}{\begin{tabular}[c]{@{}c@{}}Model\\ Ensemble\end{tabular}}            & TreeEns   & Tree Ensemble                            \\
                                                                               &                                                                                      & DeepEns   & Deep Ensemble                            \\
                                                                               &                                                                                      & HeteroEns & Heterogeneous Ensemble                   \\ \cmidrule(r){2-4}
                                                                               &                                                                                      & NAT       & Naive Adversarial Training               \\
                                                                               & \multirow{3}{*}{MA-AT}                                                               & Avg-AT   & Average Ensemble AT                                          \\
                                                                               &                                                                                      & Max-AT   & Maximize Ensemble AT                                         \\
                                                                               &                                                                                      & R-AT   & Robust Ensemble AT                                         \\ \cmidrule(r){3-4}
                                                                               &                                                                                      & TE-AT   & Transfer Ensemble AT                                         \\ \cmidrule(r){2-4}
    \multirow{7}{*}{\begin{tabular}[c]{@{}c@{}}\textbf{Utility} \\ \textbf{Metrics}\end{tabular}} & \multirow{3}{*}{Attacks}                                          & $ASR$       & Attack Success Rate                      \\
                                                                               &                                                                                      & $ASR_{avg}$  & Average Attack Success Rate                                        \\ \cmidrule(r){2-4}
                                                                               & \multirow{4}{*}{Defenses}                                                            & $DSR$       & Defense Success Rate                     \\
                                                                               &                                                                                      & $DSR_{avg}$  & Average Defense Success Rate                                          \\
                                                                               &                                                                                      & $ODR$       & Original Detection Rate                  \\ \cmidrule(l){1-4} 
    \end{tabular}
\end{center}
    \end{table}

\section{Adversarial Attack Algorithms}
\label{sec-app-attack}
\subsection{Gradient-based Attacks.}

\subsubsection{Fast Gradient Sign Method (FGSM).}
To facilitate the search for AEs, Goodfellow et al. \cite{goodfellow2014explaining} proposed a fast method for generating AEs called FGSM.
They perform only one step of gradient update along with the sign direction of the gradient at each pixel.
Their perturbation can be expressed as: $\eta=\epsilon \operatorname{sign}\left(\nabla_{x} L_{\theta}(x, y)\right)$.
The magnitude of the perturbation is small enough imperceptible, and $y$ is the target label.
Therefore, the generated adversarial instance $\hat{x}$ is calculated as: $\hat{x}=x+\eta$.

\subsubsection{Projected Gradient Descent (PGD).}
Madry et al. \cite{madry2017towards} proposed the use of PGD method to solve the linear assumption problem in FGSM \cite{goodfellow2014explaining}. 
PGD is an iterative attack. 
Compared with ordinary FGSM, which only performs one iteration, PGD performs multiple iterations.
Each time a small step is taken, each iteration will project the perturbation within the specified range.
Specifically, the gradient of the loss with respect to the input at time $t$ is expressed by:
\begin{equation}
g_t=\nabla_{x_t}(L(f_\theta(x_t), y))    
\end{equation}
The adversarial input at time $t+1$ is calculated from the input and the gradient at time $t$, i.e., 
\begin{equation}
    x_{t+1}=\prod_{x+\delta}(x_t+\epsilon(g_t/\Vert g_t\Vert))
\end{equation}

\subsubsection{Carlini and Wagner Attack (C\&W).}
Carlini and Wagner \cite{carlini2017towards} proposed an optimization-based attack method named C\&W.
The optimization function is defined as the distance between the clean example $x$ and the adversarial example $x+\delta$, i.e.,
\begin{equation}
    \min l(x, x+\delta)
\end{equation}
$$
\begin{aligned}
& s.t. & f(x+\delta)=t &\\
& & x+\delta\in[0, 1]^n &
\end{aligned}$$
where $f$ and $t$ represent the output and target label.
The C\&W attack considers both high attack accuracy and low adversarial perturbation.
On the basis of minimizing the distance metric, the probability of model misclassification is improved.

\subsubsection{DeepFool Attack (DF).}
Moosavi-Dezfooli et al.\cite{moosavi2016deepfool} proposed the DeepFool adversarial method to find the closest distance from the original input to the decision boundary of AEs.
DeepFool is an untargeted attack technique optimized for the $l_2$ distance metric.
An iterative attack by linear approximation is proposed in order to overcome the nonlinearity at a high dimension.
If $f$ is a binary differentiable classier, an iterative method is used to approximate the perturbation by considering that $f$ is linearized around $x + r$ in each iteration.
The minimal perturbation is provided by:
\begin{equation}
       \arg _{r} \min \left(\|r\|_{2}\right) \text { s.t. } f(x+r)+\nabla_{x} f(x+r)^{T} * r=0
\end{equation}
This result can be extended to a more general $l_p$ norm.

\subsubsection{Basic Iterative Method (BIM).}
The BIM attack\cite{kurakin2016adversarial} is an iterative version of FGSM where a small perturbation is added in each iteration.
There are two versions of BIM attack: BIM-A and BIM-B.
The BIM-A method stops the iteration as soon as misclassification is achieved.
In the BIM-B method, iterations only stop after a fixed number of rounds.

\subsubsection{Jacobian-based Saliency Map (JSMA).}
JSMA \cite{papernot2016limitations} is an iterative method that achieves misclassification of an input to any pre-specified class.
It uses feature selection with the aim of minimizing the number of features perturbed.
The adversary computes the Jacobian of the model:$\left[\frac{\partial f_{j}}{\partial x_{i}}(x)\right]_{i, j}$ where component $(i,j)$ is the derivative of class $j$ with respect to input feature $i$.
To compute the adversarial saliency map, the adversary then computes the following for each input feature $i$:
\begin{equation}
       S(x, t)[i]=\left\{\begin{array}{l}
       0 \quad \text { if } \frac{\partial f_{t}(x)}{\partial x_{i}}<0 \text { or } \sum_{j \neq t} \frac{\partial f_{j}(x)}{\partial x_{i}}>0 \\
       \frac{\partial f_{t}(x)}{\partial x_{i}}\left|\sum_{j \neq t} \frac{\partial f_{j}(x)}{\partial x_{i}}\right| \quad \text { otherwise }
       \end{array}\right.
\end{equation}
where $t$ is the target class that the adversary wants the machine learning model to assign.

\subsection{Gradient-free attacks.}
The next step is to introduce six gradient-free attacks.

\subsubsection{Zeroth-order optimization (ZOO).}
The zeroth-order optimization (ZOO) attack was presented in Chen et al.\cite{chen2017zoo}.
ZOO uses hinge loss in Equation:
\begin{equation}
       \max \left(\arg _{i \neq t} \max (\log (f(x+r, i)))-\log (f(x+r, t)),-k\right)
       \end{equation}
where the input $x$, correctly classified by the classifier $f$ , is perturbed with $r$, such that the resulting adversarial example is $x+r$.
ZOO uses the symmetric difference quotient to estimate the gradient and Hessian:
\begin{equation}
       \begin{array}{c}
       \frac{\partial f(x)}{\partial x_{i}} \approx \frac{f\left(x+h * e_{i}\right)-f\left(x-h * e_{i}\right)}{2 h} \\
       \frac{\partial^{2} f(x)}{\partial x_{i}^{2}} \approx \frac{f\left(x+h * e_{i}\right)-2 f(x)+f\left(x-h * e_{i}\right)}{h^{2}}
       \end{array}
       \end{equation}
where $e_i$ denotes the standard basis vector with the i-th component as 1, and $h$ is a small constant.

\subsubsection{Natural Evolutionary Strategies (NES).}
To estimate the gradient, Ilyas et al. \cite{ilyas2018black} use Natural Evolutionary Strategies (NES), a method for derivative-free optimization based on the idea of a search distribution $\pi(\theta|x)$.
Rather than maximizing an objective function $L(x)$ directly, NES maximizes the expected value of the loss function under the search distribution.
Ilyas et al. employ antithetic sampling to generate a population of $\delta_i$ values: instead of generating $n$ values $\delta_{i} \sim \mathcal{N}(0, I)$, 
they sample Gaussian noise for $i \in\left\{1, \ldots, \frac{n}{2}\right\}$ and set $\delta_{j}=-\delta_{n-j+1}$ for $j \in\left\{\left(\frac{n}{2}+1\right), \ldots, n\right\}$.
Evaluating the gradient with a population of $n$ points sampled under this scheme yields the following variancereduced gradient estimate:
\begin{equation}
       \nabla \mathbb{E}[L(\theta)] \approx \frac{1}{\sigma n} \sum_{i=1}^{n} \delta_{i} L\left(\theta+\sigma \delta_{i}\right)
\end{equation}

\subsubsection{Zeroth-Order Stochastic Gradient Descent (ZOSGD).}
Ghadimi et al. \cite{ghadimi2013stochastic} aim to estimate the gradient $\triangledown_\mathbf{x}g(\mathbf{x})$ of the ML model $f'$ more accurately to generate adversarial feature $\hat{\mathbf{x}}$.
ZOSGD gradient estimation is constructed by forward comparing two function values at random directions: 
$\nabla_\mathbf{x}g(\mathbf{x})=(1/ \sigma)[g(\mathbf{x}+\sigma\mathbf{u})-g(\mathbf{x})] \mathbf{u}$, 
where $\mathbf{u}$ is a random vector drawn uniformly from the sphere of a unit ball, and $\sigma> 0$ is a small step size, known as the smoothing parameter. 
The random direction vector $\mathbf{u}$ is drawn from the standard Gaussian distribution.
We evaluate the gradient with a population of $q$ points sampled under this scheme:
\begin{equation} 
\nabla \mathbb{E}[g(\mathbf{x})] \approx \frac{1}{\sigma q} \sum_{i=1}^{q} \mathbf{u}_{i} [g\left(\mathbf{x}+\sigma \mathbf{u}_{i}\right)-g(\mathbf{x})].
\end{equation}

\subsubsection{Zeroth-Order Adaptive Momentum Method (ZOAdaMM).}
The adaptive momentum method (AdaMM) \cite{chen2019zo}, which uses past gradients to update descent directions and learning rates simultaneously, has become one of the most popular first-order optimization methods for solving machine learning problems.
In this paper, we propose a zeroth-order AdaMM (ZO-AdaMM) algorithm, that generalizes AdaMM to the gradient-free regime.

\subsubsection{HopSkipJumpAttack (HSJA).}
Chen et al. \cite{chen2020hopskipjumpattack} described an optimization framework for finding adversarial instances for an $m$-ary classification model of the following type.
The first component is a discriminant function $F : \mathbb{R}_d\rightarrow \mathbb{R}_m$ that accepts an input $x \in [0:1]^d$ and produces an output $y \in \Delta_{m}:=\left\{y \in[0,1]^{m} \mid \sum_{c=1}^{m} y_{c}=1\right\}$.
The output vector $y=\left(F_{1}(x), \ldots, F_{m}(x)\right)$ can be viewed as a probability distribution over the label set $[m]=\{1, \ldots, m\}$.
Based on the function $F$, the classifier $C: \mathbb{R}^{d} \rightarrow[m]$ assigns input $x$ to the class with maximum probability—that is,
\begin{equation}
       C(x):=\arg \max _{c \in[m]} F_{c}(x)
       \end{equation}
Formally, if we define the function $S_{x^{\star}}: \mathbb{R}^{d} \rightarrow \mathbb{R}$ via
hen a perturbed image $x'$ is a successful attack if and only if $S_{x^\ast} (x') > 0$.

\subsubsection{Boundary Attack (BA).}
In order to search for the AEs with the minimum distance from the original example, the BA algorithm \cite{brendel2017decision} uses a strategy that performs a random walk at the decision boundary of the target detector, constantly searching for a better example.
The algorithm selects a random AE $\hat{x_0}$ as the initial point, which can be misclassified by the target detector but is not guaranteed to have the minimum distance from the original sample;
The algorithm then performs $t$ iterations, in which in each iteration, the algorithm extracts a random perturbation $\delta_t$ from a certain distribution and adds it to the previous AE $\hat{x_t}$, updating the AE.
If $\hat{x_t}+\delta_t$ is adversarial, and continuing to extract the perturbation in the opposite direction.
