# Supplementary material for: CARE: Ensemble Adversarial Robustness Evaluation Against Adaptive Attackers for Security Applications
Source: arXiv:2401.11126 source file (2024-01-20)
Supplement: Supplementary file 2 [file 9-appendix-bayesopt.tex]

\section{Bayesian Optimization}
\label{sec-app-bayesopt}
We detail the Gaussian process and acquisition function here.

\subsection{Gaussian Process}
When sampling is viewed as sampling a function, and after understanding that sampling an infinite dimension is equivalent to sampling a function, the original probability density function ceases to be a distribution of points, but becomes a distribution of functions. 
This infinite elementary Gaussian distribution is called a Gaussian process.
A Gaussian process is formally defined as: for all $\boldsymbol{x}=\left[x_{1}, x_{2}, \cdots, x_{n}\right], f(\boldsymbol{x})=\left[f\left(x_{1}\right), f\left(x_{2}\right), \cdots, f\left(x_{n}\right)\right]$ , which obey a multivariate Gaussian distribution, denoted as
\begin{equation}
       f(\boldsymbol{x}) \sim \mathcal{N}(\boldsymbol{\mu}(\boldsymbol{x}), \kappa(\boldsymbol{x}, \boldsymbol{x}))
       \end{equation}
Here $\mu(x): \mathbb{R}^{n} \rightarrow \mathbb{R}^{n}$ represents the Mean function, which returns the mean of each dimension; $\kappa(\boldsymbol{x}, \boldsymbol{x}): \mathbb{R}^{\mathbf{n}} \times \mathbb{R}^{\mathbf{n}} \rightarrow \mathbb{R}^{\mathbf{n} \times \mathbf{n}}$ is the Covariance Function (also called the Kernel Function) returns the covariance matrix between the dimensions of the two vectors.
% For a Gaussian process, a mean function and a covariance function are uniquely defined, and a finite subset of dimensions has a multivariate Gaussian distribution.

\subsection{Acquisition Function}
Acquisition functions are designed in order to make each sample as close to the maximum/minimum value of the target function as possible, thus making locating extreme value points more efficient.
Specifically, we use $\mathcal{U}(\mathbf{x})$ to denote the sampling function for a given GP model, and for the next sampling of the target function
\begin{equation}
       \mathbf{x}_{*}=\arg \max _\mathbf{x} \mathcal{U}(\mathbf{x})
       \end{equation}
A GP model is given as the mean $\mu(\mathbf{x})$ and variance $\sigma (\mathbf{x})$ of the objective function, and a straightforward strategy is to choose points with a greater probability than the objective function value for the current observations (assuming we are looking for the extreme values), 
Thus, $f\left(\mathbf{x}^{+}\right)$ is the maximum value of the current observations, and the sampling function can be found
\begin{equation}
       \begin{aligned}
       P I(\mathbf{x}) &=p\left(f(\mathbf{x}) \geq f\left(\mathbf{x}^{+}\right)\right) \\
       &=\Phi\left(\frac{\mu(\mathbf{x})-f\left(\mathbf{x}^{+}\right)}{\sigma(\mathbf{x})}\right)
       \end{aligned}
       \end{equation}
where $\Phi(\cdot)$ is the standard normal cumulative distribution function.
But the acquisition function we chose is GP-UCB.

\textbf{Upper confidence bound (UCB $\&$ GP-UCB).}
UCB consists of a component $\mu(\mathbf{x})$ that reflects expected return and a component $\kappa \sigma(\mathbf{x})$ that reflects risk and controls exploration through the parameter $\kappa$.
In GP-UCB \cite{srinivas2009gaussian}, $\beta_{t}$ varies with sampling progress $t$.
\begin{equation}
       \begin{aligned}
       U C B(\mathbf{x}) &=\mu(\mathbf{x})+\kappa \sigma(\mathbf{x}), \quad \kappa>0 \\
       G P-U C B(\mathbf{x}) &=\mu(\mathbf{x})+\sqrt{\beta_{t}} \sigma(\mathbf{x})
       \end{aligned}
       \end{equation}
Original paper used the following equation experimentally:
\begin{equation}
       \beta_{t}=2 \log \left(|D| t^{2} \pi^{2} / 6 \delta\right), \quad \delta \in(0,1)
\end{equation}
